# Supplementary material for: FedGTST: Boosting Global Transferability of Federated Models via Statistics Tuning
Source: arXiv:2410.13045 source file (2024-10-16)
Supplement: Supplementary file 1 [file Appendix.tex]

\newpage
\begin{center}
\textbf{Appendix}    
\end{center}

%Proof: lemma: federated Round-wise upper bound

\begin{lemma}[Lemma \ref{lem:gnr-ub}]
Assume that $l:\gW_h\times\gP_{\gX\times\gY}\to \sR_+$ is convex w.r.t. $w_{h}$. 
\begin{align*}
    L_{\gD_S}(h_S^{(0)})\leq \sE_{k\in[K]}\big[L_{\gD_S^{(k)}}\big(h_S^{(k)}\big)\big] + \overline{d}_{\gH}(\gD_S),
\end{align*}
where $\overline{d}_{\gH}(\gD_S):= \sE_{i,j\in[K]}d_{\gH}(\gD_S^{(i)}, \gD_S^{(j)})$.
\end{lemma}

\begin{proof}
\begin{align*}
    L_{\gD_S}(h) &= \fK\sum_{k\in[K]} L_{\gD_S^{(k)}}(h_{S}^{(0)})\\
    & = \fK\sum_{k\in[K]} \sE_{(x,y)\sim \gD_S^{(k)}}l(h(x,w_{h,S}^{(0)}),y)\\
    & = \fK\sum_{k\in[K]} \sE_{(x,y)\sim \gD_S^{(k)}}l(h(x,\fK\sum_{i\in[K]}w_{h,S}^{(i)}),y)\\
    &\leq \frac{1}{K^2}\sum_{\substack{k\in[K]\\i\in [K]}} \sE_{(x,y)\sim \gD_S^{(k)}}l(h(x,w_{h,S}^{(i)}),y)\\
    &= \frac{1}{K^2}\sum_{\substack{k\in[K]\\i\in [K]}} L_{\gD_S^{(k)}}(h_{S}^{(i)})\\
    & \leq \frac{1}{K^2}\sum_{\substack{k\in[K]\\i\in [K]}} \big[L_{\gD_S^{(i)}}(h_{S}^{(i)}) + d_{\gH}(\gD_S^{(i)}, \gD_S^{(k)})\big]\\
    & = \fK\sum_{i\in [K]}L_{\gD_S^{(i)}}(h_{S}^{(i)}) + \frac{1}{K^2}\sum_{\substack{i\in [K]\\j\in[K]}}d_{\gH}(\gD_S^{(i)}, \gD_S^{(j)})\\
    & = \sE_{k\in[K]}L_{\gD_S^{(k)}}(h_{S}^{(k)})+\overline{d}_{\gH}(\gD_S)
\end{align*}
\end{proof}

\begin{lemma}[Lemma \ref{lem:round-ub}]
With Assumption \ref{asp:one-GD} and \ref{asp:ltz-grad}, define the domain-wise expected Jacobian matrix of loss $l$ w.r.t $w_h$ as $J_l^{(i)}(w'):= \sE_{(x,y)\in \gD_S^{(i)}} \nabla_{w} l(h(x,w_h),y)\big|_{w_h = w'}$. Denote learning rate of agent $(i)$ at round $p$ as $\overline{\lambda}^{p}$ 
\begin{align*}
    L_{\gD_S}(h_S^{(0),p+1})\leq L_{\gD_S}(h_S^{(0),p})
    -
    \beta_1({\lambda}^{p+1})\cdot
    \|J_l^p\|_2^2 + 
     \beta_2({\lambda}^{p+1})\cdot
    \|\delta (J_l^{p})\|_2^2
\end{align*}
where $\beta_1(\lambda) := {\lambda} - \beta_2(\lambda)$; 
$\beta_2(\lambda) := \frac{\alpha{\lambda}^2}{2}$; $\overline{\lambda}:=\frac{}{}$ ; $J_l^p:= \sE_{i\in[K]}J_l^{(i)}(w_{h,S}^{(i),p})$
\end{lemma}

\begin{proof}
\begin{align*}
L_{\gD_S}(h_S^{(0),p+1}) 
&\leq \frac{1}{K^2}\sum_{\substack{k\in[K]\\i\in[K]}}L_{\gD_S^{(k)}}(h_S^{(i),p+1})
\end{align*}

\begin{align*}
L_{\gD_S^{(k)}}\big(h_S^{(i),p+1}\big)
&=\sE_{(x_k,y_k)\in\gD_S^{(k)}}l(h(x_k,w_{h,S}^{(i),p+1}),y_k)
\end{align*}

\begin{align*}
l(h(x_k,w_{h,S}^{(i),p+1}),y_k)
& =  l\bigg(h\big(x_k,w_{h,S}^{(0),p} - \lambda^{(i),p+1}\cdot
\big[\nabla_w L_{\gD_S^{(i)}}(h_S^{(0),p})\big|_{w = w_{h,S}^{(0),p}}\big]\big),y_k\bigg)\\
& =  l\bigg(h\big(x_k,w_{h,S}^{(0),p} - \lambda^{(i),p+1}\cdot
\big[\nabla_w 
\sE_{(x_i,y_i)\sim \gD_S^{(i)}}l(h(x_i,w),y_i)
\big|_{w = w_{h,S}^{(0),p}}\big]\big),y_k\bigg)\\
& =  l\Bigg(h\bigg(x_k,w_{h,S}^{(0),p} - \lambda^{(i),p+1}\cdot
J_l^{(i)}\big(w_{h,S}^{(0),p}\big)\bigg),y_k\Bigg)
\end{align*}

Let $\Delta := -\lambda^{(i),p+1}\cdot
J_l^{(i)}\big(w_{h,S}^{(0),p}\big)$

\begin{align*}
l(h(x_k,w_{h,S}^{(i),p+1}),y_k)
& = l\Bigg(h\bigg(x_k,w_{h,S}^{(0),p} +\Delta\bigg),y_k\Bigg)\\
& \leq l\Big(h\big(x_k,w_{h,S}^{(0),p} \big),y_k\Big) +\bigg[\nabla_w  l\Big(h\big(x_k,w \big),y_k\Big)\big|_{w = w_{h,S}^{(0),p}}\bigg]^\top \cdot\Delta + \frac{\alpha}{2}\Delta^\top\Delta\\
\end{align*}

\begin{align*}
    L_{\gD_S^{(k)}}\big(h_S^{(i),p+1}\big)
&=\sE_{(x_k,y_k)\in\gD_S^{(k)}}l(h(x_k,w_{h,S}^{(i),p+1}),y_k)\\
&\leq \sE_{(x_k,y_k)\in\gD_S^{(k)}}
\Bigg[\Big(h\big(x_k,w_{h,S}^{(0),p} \big),y_k\Big) +\bigg[\nabla_w  l\Big(h\big(x_k,w \big),y_k\Big)\big|_{w = w_{h,S}^{(0),p}}\bigg]^\top \cdot\Delta + \frac{\alpha}{2}\Delta^\top\Delta\Bigg]\\
& = L_{\gD_S^{(k)}}(h_{S}^{(0),p}) + \big[J_l^{(k)}(w_{h,S}^{(0),p})\big]^\top\cdot\Delta + \frac{\alpha}{2}\Delta^\top\Delta
\end{align*}

\begin{align*}
L_{\gD_S}(h_S^{(0),p+1}) 
\leq &\frac{1}{K^2}\sum_{\substack{k\in[K]\\i\in[K]}}
L_{\gD_S^{(k)}}(h_S^{(i),p+1})\\
\leq & \frac{1}{K^2}\sum_{\substack{k\in[K]\\i\in[K]}}
\Bigg[L_{\gD_S^{(k)}}(h_{S}^{(0),p}) + \big[J_l^{(k)}(w_{h,S}^{(0),p})\big]^\top\cdot\Delta + \frac{\alpha}{2}\Delta^\top\Delta\Bigg]\\
=& \frac{1}{K^2}\sum_{\substack{k\in[K]\\i\in[K]}}
\Bigg[L_{\gD_S^{(k)}}(h_{S}^{(0),p}) 
- \lambda^{(i),p+1}\cdot\big[J_l^{(k)}(w_{h,S}^{(0),p})\big]^\top\cdot\big[
J_l^{(i)}\big(w_{h,S}^{(0),p}\big)\big] + \\
&\frac{\alpha}{2}\cdot(\lambda^{(i),p+1})^2\cdot\|
J_l^{(i)}\big(w_{h,S}^{(0),p}\big)\|_2^2\Bigg]\\
=&L_{\gD_S}(h_{S}^{(0),p}) - \sE_{i\in[K]}\Big[\lambda^{(i),p+1}\cdot J_l^{(i)}\big(w_{h,S}^{(0),p}\big)\Big]^\top\cdot J_l^p +  \frac{\alpha}{2}\sE_{i\in [K]} (\lambda^{(i),p+1})^2\cdot\|
J_l^{(i)}\big(w_{h,S}^{(0),p}\big)\|_2^2
\end{align*}

When $\lambda^{(i),p} = \lambda^{p}, \forall i\in[K], p\in [P]$,

\begin{align*}
L_{\gD_S}(h_S^{(0),p+1}) 
\leq&L_{\gD_S}(h_{S}^{(0),p}) - \lambda^{p+1}\|J_l^p\|_2^2 
+  (\lambda^{p+1})^2\cdot \frac{\alpha}{2}\sE_{i\in [K]} \|
J_l^{(i)}\big(w_{h,S}^{(0),p}\big)\|_2^2
\end{align*}

Let $\sigma^2_{J,p} := \sE_{i\in [K]} \|
J_l^{(i)}\big(w_{h,S}^{(0),p}\big)\|_2^2 - \|
\sE_{i\in [K]} J_l^{(i)}\big(w_{h,S}^{(0),p}\big)\|_2^2
=\sE_{i\in [K]} \|
J_l^{(i)}\big(w_{h,S}^{(0),p}\big)\|_2^2 - \|
J_l^p\|_2^2
$,

\begin{align*}
L_{\gD_S}(h_S^{(0),p+1}) 
\leq&L_{\gD_S}(h_{S}^{(0),p}) - \lambda^{p+1}\|J_l^p\|_2^2 
+  (\lambda^{p+1})^2\cdot \frac{\alpha}{2}(\sigma^2_{J,p} + \|J_l^p\|_2^2)\\
= &L_{\gD_S}(h_{S}^{(0),p}) 
- (\lambda^{p+1}
- \frac{\alpha\cdot(\lambda^{p+1})^2}{2})\|J_l^p\|_2^2 
+  \frac{\alpha\cdot(\lambda^{p+1})^2}{2}\sigma^2_{J,p}\\ 
= &L_{\gD_S}(h_{S}^{(0),p}) 
- \beta_1(\lambda^{p+1})\|J_l^p\|_2^2 
+  \beta_2(\lambda^{p+1})\sigma^2_{J,p}
\end{align*}

\end{proof}
